# Supplementary material for: Multimodal Fusion Network for Micro-displacement Measurement via Michelson Interferometer
Source: arXiv:2511.12192 source file (2026-03-16)
Supplement: Supplementary file 1 [file Supplemental_Document.pdf]

# Supplemental Document

ZIXING JIA, JIAWEI LI, ZIPING CHEN, XIN LI

## 1. DETAILED EXPLANATION OF INPUT FEATURES

### A. Image Channels

Given a single grayscale interferometric frame  $I_t(x, y)$  at time  $t$ , we derive the following three 2D inputs:

**(1) Original Interferogram** The original image  $I_t$  itself is directly used as a spatial-phase carrier:

$$I_{\text{orig}}(x, y) = I_t(x, y) \quad (\text{S1})$$

This retains the raw fringe structure, which contains phase shift information induced by displacement.

**(2) Frame Difference Image** If a previous frame  $I_{t-1}$  is available, we compute the pixel-wise absolute difference:

$$I_{\text{diff}}(x, y) = |I_t(x, y) - I_{t-1}(x, y)| \quad (\text{S2})$$

This highlights localized intensity changes, capturing dynamic variations as voltage modulates displacement.

**(3) Frequency-Domain Image via FFT** We compute the magnitude spectrum of the 2D Fourier Transform (after centering and log-scaling):

$$I_{\text{fft}}(u, v) = \frac{\log(|\mathcal{F}[I_t](u, v)| + \epsilon) - \min}{\max - \min} \quad (\text{S3})$$

where  $\mathcal{F}$  denotes the centered 2D FFT, and normalization ensures bounded values. This captures periodic frequency features corresponding to fringe spacing and order.

### B. Numerical Channels

In addition to image-based inputs, we extract seven scalar features  $\mathbf{f} \in \mathbb{R}^7$  from  $I_t$ , each providing a compact statistical or physical cue:

**(1) Normalized Frame Index**

$$f_1 = \frac{t}{T-1} \quad (\text{S4})$$

where  $T$  is the total number of frames. This encodes sequence context[1].

**(2) Mean Intensity**

$$f_2 = \frac{1}{HW} \sum_{x=1}^H \sum_{y=1}^W I_t(x, y) \quad (\text{S5})$$

representing average brightness.  $H$  and  $W$  stand for height and width.

**(3) Intensity Variance**

$$f_3 = \frac{1}{HW} \sum_{x,y} (I_t(x, y) - f_2)^2 \quad (\text{S6})$$

captures contrast and fringe clarity. Mean intensity ( $f_2$ ) and intensity variance ( $f_3$ ) serve as simple but informative image-quality / fringe-contrast statistics and have been widely used in image-quality and fringe-analysis studies.[2]

**(4) Number of Horizontal Fringe Peaks** Let  $P(y)$  be the horizontal mean intensity:

$$P(y) = \frac{1}{H} \sum_{x=1}^H I_t(x, y), \quad f_4 = \text{PeakCount}(P(y)) \quad (\text{S7})$$

measuring spatial frequency through ridge counts.

**(5) Low-Frequency Energy Ratio** Let  $\hat{I}(u, v)$  be the FFT magnitude spectrum, and  $M$  a circular mask centered at  $(u_0, v_0)$ :

$$f_5 = \frac{\sum_{(u,v) \in M} |\hat{I}(u, v)|^2}{\sum_{(u,v)} |\hat{I}(u, v)|^2} \quad (\text{S8})$$

quantifies how much energy resides in low-frequency bands.[3, 4]

**(6) Spectral Centroid Distance** The spectral center of mass:

$$f_6 = \sqrt{(\bar{u} - u_0)^2 + (\bar{v} - v_0)^2}, \quad \bar{u} = \frac{\sum_u u \cdot \sum_v \hat{I}(u, v)}{\sum_{u,v} \hat{I}(u, v)} \quad (\text{S9})$$

describes the frequency bias (higher values imply more rapid fringe changes). The spectral centroid distance  $f_6$  gives a noise-robust indicator of shifts in dominant fringe frequency, as used in signal/spectral analysis literature.[5]

**(7) Image Entropy** Using a normalized histogram  $p_i$  of 256 bins:

$$f_7 = - \sum_{i=1}^{256} p_i \log_2(p_i + \delta) \quad (\text{S10})$$

reflects complexity and texture richness. Image entropy  $f_7$  serves as a compact measure of image information/texture and has been used as a quality / sensitivity metric in optical sensing and fringe/ speckle analyses.[6].

## 2. PRE-TRAIN MODEL ACCURACY EVALUATION

All displacement prediction accuracies reported in this work are expressed in terms of the root mean square error (RMSE), and all uncertainty values correspond to Type-A standard uncertainties unless otherwise specified. The Type-A uncertainty  $u_A$  was evaluated as the standard deviation of repeated RMSE measurements under identical experimental conditions:

$$u_A = \sqrt{\frac{\sum_{i=1}^N (x_i - \bar{x})^2}{N(N-1)}}, \quad (\text{S11})$$

where  $x_i$  denotes the RMSE obtained from the  $i$ -th independent measurement,  $\bar{x}$  is the mean RMSE, and  $N$  is the number of repeated samples.

In the main text, the pre-trained model accuracy is reported in two contexts:

- **Overall model precision (Abstract):** The model achieves an average displacement prediction accuracy of  $4.84 \pm 0.15$  nm. Here, the RMSE value represents the mean of ten independent training batches, and the quoted uncertainty ( $\pm 0.15$  nm) corresponds to the Type-A uncertainty calculated with  $N = 10$  according to Eq. (S11).
- **Noise robustness analysis (Section Results and Discussion):** In the comparative experiments under different noise intensities, each noise level was evaluated across ten independent folders of simulated interferograms. The reported RMSE for each noise condition is the mean over these ten subsets, and the associated Type-A uncertainty was computed with  $N = 10$  in the same manner.

All accuracy results in the paper and supplementary materials thus follow a consistent definition:

$$\text{Reported Accuracy} = \bar{x} \pm u_A, \quad (\text{S12})$$

where  $\bar{x}$  is the mean RMSE and  $u_A$  is the corresponding Type-A standard uncertainty estimated from ten repeated trials. This ensures statistical comparability across experiments and provides a reliable measure of model precision under both nominal and noisy imaging conditions.

### 3. PIEZOELECTRIC ACTUATOR AND VOLTAGE–DISPLACEMENT CONVERSION

The piezoelectric actuator employed in our experiments is the **PST150/2x3/10** model (CoreMorrow Inc.), with official specifications available online<sup>1</sup>. Due to prolonged usage of the device, we recalibrated its displacement characteristics prior to experimentation. The measured performance indicates a maximum displacement of approximately 6000 nm under a maximum driving voltage of +120 V.

For voltage control, we utilized an **NI myDAQ** system<sup>2</sup> as the signal generator. The output unit of NI myDAQ is in millivolts (mV), which was subsequently amplified 24 times by a voltage amplifier before being applied to the piezoelectric actuator. Based on the recalibrated displacement range, the conversion relationship between the myDAQ output voltage and the estimated displacement increment  $\Delta$  (in nanometers) between two consecutive interferometric images is given by:

$$\Delta \text{ (nm)} = V_{\text{myDAQ}} \times 0.001 \times \frac{6000}{120}, \quad (\text{S13})$$

where  $V_{\text{myDAQ}}$  denotes the output voltage from the NI myDAQ in units of millivolts. This linear calibration ensures that each step in applied voltage can be precisely mapped to an estimated nanoscale displacement, enabling accurate correlation between interferogram sequences and actuator motion.

### 4. DETAILED EXPLANATION OF EXPERIMENT

#### A. Experimental Instrumentation

The measurement scheme is implemented in Python using a nested loop structure:

- **Zero level:** loop involves sweeping the voltage from the starting point of the sliding window ('StartV') to its end point, under a fixed voltage step size ('Step') and a fixed sliding window length ('WindowLength').
- **First Level: Variation of Step Size ('Step').** The step size is varied from 0.6V to 19.2V, with an increment of 0.6V per iteration.
- **Second Level: Shifting of the Acquisition Window ('StartV').** The starting point of the sliding window is shifted across the range from  $[0, L_0 + L_{\text{var}}]$  V to  $[100.8 - (L_0 + L_{\text{var}}), 100.8]$  V. The shift increment for each step is 1.008 V.
- **Third Level: Adjustment of the Window Length ('WindowLength').** The length of the sliding window is adjusted within the range of  $[50.4, 100.8]$  V.

#### B. Possible Noise Analysis of the Experiment

To measure the background noise of the Michelson interferometer, we employed the HAA algorithm to estimate its approximate displacement from images. A comparison between the fitted image and the original (unfiltered) image is shown in Figure S1. According to the measurement protocol, the error associated with each measurement set is statistically independent. Therefore, our primary concern is the cumulative error over a given time interval. The characteristic time of 50 s corresponds to the longest duration among all our measurement sets. Figure 2 presents the noise observed when the interferometer remained stationary over the 0–50 s interval, exhibiting a standard deviation of 0.3 nm. However, it should be noted that residual noise sources prevent the fitting procedure from fully capturing the true displacement. After conducting 12 independent measurements across different time intervals, we conservatively estimate that the standard deviation of the stationary noise does not exceed 10 nm.

The static noise performance of the CAP capacitive sensor is shown in Fig. S3. The measured displacement exhibits a standard deviation of 14 nm under stationary conditions. Compared to the absolute displacement  $d$ , the differential displacement  $\Delta d = d_{i+1} - d_i$  is of primary interest in this work. Assuming that the dominant noise source is the static sensor noise, and that successive measurements are uncorrelated, the standard deviation of  $\Delta d$  is obtained via error propagation:

$$\sigma_{\Delta d} = \sqrt{\sigma^2 + \sigma^2} = \sqrt{2} \sigma \approx \sqrt{2} \times 14.1 \text{ nm} \approx 19.9 \text{ nm}. \quad (\text{S14})$$

<sup>1</sup><http://www.coremorrow.com/proshow-9-168-1.html>

<sup>2</sup><https://www.ni.com/zh-cn/shop.html#pinned-nav-section1>

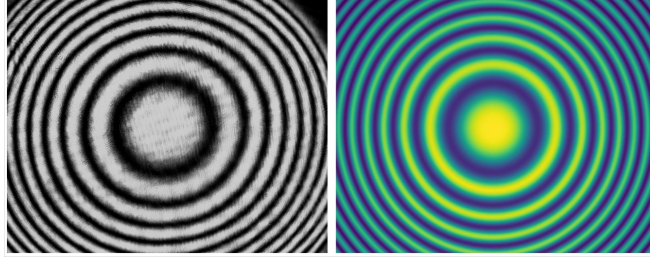

**Fig. S1.** (Left) Raw interferogram captured by the CCD camera.(Right) Reconstructed interferogram obtained using the HAA-based fringe fitting model.

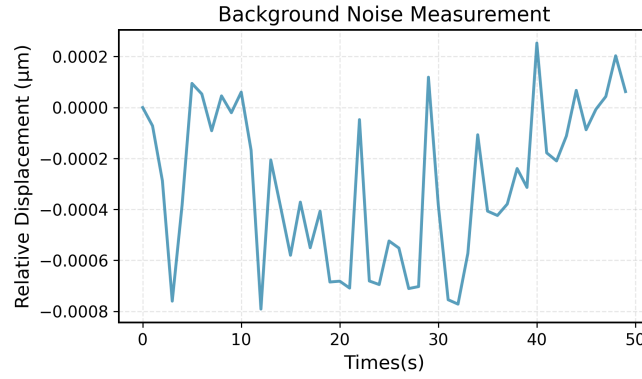

**Fig. S2.** Optical path difference (OPD) drift of the Michelson interferometer from 0 to 50 s, with displacement obtained via HAA-based phase fitting

However, it should be noted that the sensor operates by forming a capacitance between the probe and the target surface; consequently, measurement uncertainty increases significantly during dynamic operation. Although the acquisition frequency in our experiments was limited to below 200 Hz, this dynamic error remains one of the primary factors limiting the overall displacement measurement accuracy in this study. If we assume that the instrumental error varies linearly with frequency,  $\sigma$  would reach approximately 34.6 nm under the experimental conditions as indicated in the device manual.

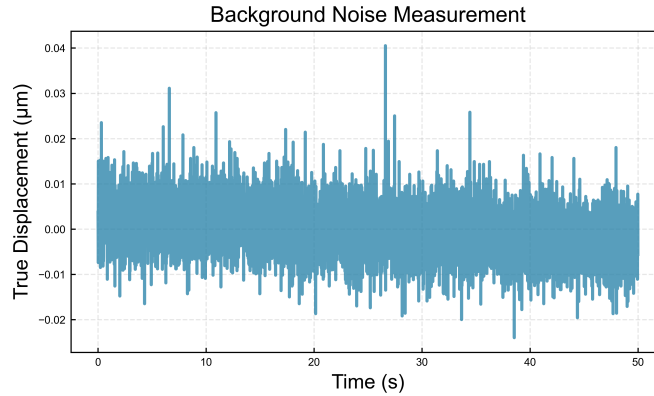

**Fig. S3.** Static displacement noise of the CAP capacitive sensor over 50s

Additional factors may also influence the experimental results. First, the large-scale training dataset (on the order of  $10^6$  samples) could potentially accelerate the aging process of the piezoelectric actuator due to prolonged and repeated actuation. Second, inherent hardware discrepancies between the optical interferometer experiment and the voltage–displacement ( $V-d$

) characterization setup—such as differences in mechanical mounting, thermal environment, or timing synchronization—can significantly compromise the simultaneity and consistency of the measurements.

In light of these practical limitations, a background noise level with a standard deviation of 50-70 nm is considered a reasonable and conservative estimate for the overall system uncertainty. Therefore, limited by our background noise of 50-70nm, when we fine-tune, the predictive accuracy of the displacement head significantly decreases, dropping from about 5nm accuracy to approximately 70nm, which is close to the background noise. However, considering that the classification head, responsible for order judgment, deals with a large displacement of about 315nm, the accuracy of the classification head is not significantly affected.

### C. Experimental Instrumentation

Table S1 summarizes the instrumentation used in this experiment, including instruments and key specifications.

**Table S1.** Key instrumentation used in the optical interferometer and piezoelectric characterization experiments.

| Instrument                    | Model / Manufacturer                      | Key Specifications                                                                                                  |
|-------------------------------|-------------------------------------------|---------------------------------------------------------------------------------------------------------------------|
| Optical platform              | SGM-4 / Shanghai Sino-Guangming Co., Ltd. | Precision mechanical stability with fine adjustment                                                                 |
| Laser source                  | He-Ne laser                               | $\lambda = 633.02\text{nm}$ , output power $\approx 2\text{mW}$ , linewidth 0.04nm(measured by a spectrum analyzer) |
| Spectrum analyzer             | Yokogawa AQ6373B                          | Used for laser wavelength calibration                                                                               |
| Convex lens                   |                                           | Focal length $f=4.5\text{mm}$                                                                                       |
| CCD camera                    | Daheng MER-130-30UM                       | Resolution: 1208×1024 pixels, pixel size: 5.2 $\mu\text{m}$ , frame rate: 30fps                                     |
| Voltage amplifier             | Custom-built                              | Gain: 24×, output range: 0-120V                                                                                     |
| Piezoelectric Ceramic         | PST150/2×3/10 / Xin-Tian Tech.            | Driven by amplified voltage signal                                                                                  |
| Digital multimeter            | Rigol DM3085E                             | 5.5-digit resolution, real-time voltage monitoring                                                                  |
| Capacitive CAP Micrometer     | CAP-series / XinTian Tech.                | Static resolution: 2.5nm, range: 300 $\mu\text{m}$                                                                  |
| DAQ system (actuator control) | NI myDAQ                                  | Analog output synchronized with image acquisition                                                                   |
| DAQ system (V-d measurement)  | NI PCI-6281                               | Sampling rate: 625kS/s for simultaneous voltage and displacement recording                                          |

## 5. HAA ALGORITHM

### Algorithm S1. Heuristic Analytical Algorithm (HAA) – Preprocessing

---

```

1: procedure PROCESSINTERFERENCESEQUENCE(Raw image sequence  $\{\mathbf{I}_{\text{raw}}^{(k)}\}_{k=0}^{N-1}$ , wavelength
    $\lambda$  (in  $\mu\text{m}$ ), scan direction  $\text{dir} \in \{\text{"up"}, \text{"down"}\}$ )
2:   Initialize empty lists:  $M \leftarrow [], \Theta \leftarrow []$ 
3:   for  $k = 0$  to  $N - 1$  do
4:      $\mathbf{I}^{(k)} \leftarrow \text{PREPROCESSIMAGE}(\mathbf{I}_{\text{raw}}^{(k)})$ 
5:     if  $\mathbf{I}^{(k)} \neq \text{null}$  then
6:        $\theta^{(k)} \leftarrow \text{FITSINGLEFRAME}(\mathbf{I}^{(k)})$ 
7:       if  $\theta^{(k)} \neq \text{null}$  then
8:          $m^{(k)} \leftarrow \theta^{(k)}[4]$ 
9:          $m^{(k)} \leftarrow m^{(k)} \bmod 1$ 
10:        Append  $m^{(k)}$  to  $M$ ,  $\theta^{(k)}$  to  $\Theta$ 
11:   if  $|M| = 0$  then
12:     return empty displacement sequence
13:   Phase unwrapping and displacement computation:
14:    $\Phi \leftarrow [M[0]], D \leftarrow [0.0]$ 
15:   for  $k = 1$  to  $|M| - 1$  do
16:      $\Delta m \leftarrow M[k] - M[k - 1]$ 
17:     if  $\text{dir} = \text{"up"}$  and  $\Delta m > 0.3$  then
18:        $\Phi[k - 1] \leftarrow \Phi[k - 1] - 1$ 
19:        $\Delta m \leftarrow \Delta m - 1$ 
20:     else if  $\text{dir} = \text{"down"}$  and  $\Delta m < -0.3$  then
21:        $\Phi[k - 1] \leftarrow \Phi[k - 1] + 1$ 
22:        $\Delta m \leftarrow \Delta m + 1$ 
23:      $\Phi[k] \leftarrow \Phi[k - 1] + \Delta m$ 
24:      $\Delta d \leftarrow |\Delta m| \cdot \frac{\lambda}{2}$ 
25:     if  $\text{dir} = \text{"up"}$  then
26:        $d_k \leftarrow D[k - 1] + \Delta d$ 
27:     else
28:        $d_k \leftarrow D[k - 1] - \Delta d$ 
29:     Append  $d_k$  to  $D$ 
30:   return  $\Theta, D$ 

31: procedure PREPROCESSIMAGE(Raw image  $\mathbf{I}_{\text{raw}}$ )
32:   if  $\mathbf{I}_{\text{raw}}$  is 3D then
33:     if 3 channels then
34:        $\mathbf{I} \leftarrow \text{mean}(\mathbf{I}_{\text{raw}}, \text{axis} = 2)$ 
35:     else if 1 channel then
36:        $\mathbf{I} \leftarrow \mathbf{I}_{\text{raw}}[:, :, 0]$ 
37:     else
38:       return null
39:   else if  $\mathbf{I}_{\text{raw}}$  is 2D then
40:      $\mathbf{I} \leftarrow \mathbf{I}_{\text{raw}}$ 
41:   else
42:     return null
43:   Downsample  $\mathbf{I}$  by factor 0.75 using bilinear interpolation
44:   Apply Gaussian smoothing ( $3 \times 3$  kernel,  $\sigma = 0.5$ )
45:   Normalize  $\mathbf{I}$  to  $[0, 1]$  via min-max scaling
46:   if image has no intensity variation then
47:     return null
48:   return  $\mathbf{I}$ 

```

---

**Algorithm S2.** Heuristic Analytical Algorithm (HAA) – Main Procedure

---

- 1: **procedure** FITSINGLEFRAME(Normalized image  $\mathbf{I} \in [0, 1]^{H \times W}$ )
- 2:   Construct coordinate grid:  $X_{ij} = j, Y_{ij} = i$
- 3:   Define radial terms:

$$r_0^2 = (X - x_0)^2 + (Y - y_0)^2, \quad r_c^2 = (X - x_c)^2 + (Y - y_c)^2$$

- 4:   Define wrapped phase:  $\text{wrap}(p) = (p \bmod 1) - 0.5$
- 5:   Model intensity:

$$\hat{I}(X, Y; \theta) = e^{-cr_c^2} \cdot I_0 \cdot \left[ 1 + V \cos \left( 2\pi \cdot \text{wrap} \left( m + ar_0^2 + br_0^4 \right) \right) \right]$$

- 6:   Parameter vector:  $\theta = [I_0, a, b, c, m, x_c, y_c, x_0, y_0, V]$
  - 7:   Enforce physical constraints:
  - 8:     (i) Centers  $(x_c, y_c, x_0, y_0)$  within image bounds
  - 9:     (ii) Parameters  $a, b, c, V$  within safe ranges
  - 10:    (iii) Variance of unwrapped phase bounded
  - 11:   Optimize  $\theta$  to minimize  $\|\mathbf{I} - \hat{\mathbf{I}}\|_F^2$  via hybrid global-local optimization
  - 12:   If optimization fails, fall back to initial guess
  - 13:   Clip all parameters to valid intervals
  - 14:   **return**  $\theta$  or null if fitting fails
- 

**REFERENCES**

1. A. Vaswani, N. Shazeer, N. Parmar, *et al.*, “Attention is all you need,” (2023).
2. Z. Wang, A. Bovik, H. Sheikh, and E. Simoncelli, “Image quality assessment: from error visibility to structural similarity,” *IEEE Transactions on Image Process.* **13**, 600–612 (2004).
3. D. J. Bone, H.-A. Bachor, and R. J. Sandeman, “Fringe-pattern analysis using a 2-D Fourier transform,” *Appl. Opt.* **25**, 1653–1660 (1986).
4. M. Takeda, H. Ina, and S. Kobayashi, “Fourier-transform method of fringe-pattern analysis for computer-based topography and interferometry,” *J. Opt. Soc. Am.* **72**, 156–160 (1982).
5. M. Massar, M. Fickus, E. Bryan *et al.*, “Fast computation of spectral centroids,” *Adv Comput. Math* **35**, 83–97 (2011).
6. E. Fujiwara, Y. T. Wu, and C. M. Cordeiro, “Entropy analysis of optical fiber specklegram sensors,” *Results Opt.* **5**, 100155 (2021).
